# Supplementary material for: e-CLIP: Large-Scale Vision-Language Representation Learning in E-commerce
Source: arXiv:2207.00208 source file (2022-08-22)
Supplement: Supplementary file 1 [file 8-appendix.tex]

\appendix

\section{Appendix}

\subsection{Part One}
dddd

\subsection{Part Two}

dddd

\section{Online Resources}

dddd
